# Supplementary material for: A Novel Spatial-Temporal Specification-Based Monitoring System for Smart Cities
Source: arXiv:2104.04904 source file (2021-04-11)
Supplement: Supplementary file 1 [file a_appendix.tex]

% \section*{Appendix A}
\section*{Appendix A: Tool for SaSTL Specification and Monitoring}
In the requirement study, we also found that many requirements are written in a very ambiguous way.  The description is at high-level and often imprecise. For example, in   
DC Air Pollutants, it says that \emph{``An emission into the atmosphere of odorous or other air pollutants from any source in any quantity and of any characteristic, and duration which is, or is likely to be injurious to the public health or welfare, or which interferes with the reasonable enjoyment of life and property is prohibited''}. It basically states an environmental requirement regarding air pollution. However, there is no quantitative definition of the emission that \emph{``is likely to be injurious to the public health or welfare, or which interferes with the reasonable enjoyment of life and property''}. Even two human beings could make different decisions for the same situation based on this requirement; the monitor cannot specify or monitor a requirement like this. On the other hand, this problem indicates the important demand for a tool to help specify city requirements formally. 

\begin{figure*}[!t]
    \centering
    \includegraphics[width = 0.8\textwidth]{Figure/tool.png}
    \caption{SaSTL Monitoring Tool}
    \label{fig:tool}
    \vspace{-1em}
\end{figure*}

 
To help and inspire users to specify requirements precisely without knowledge of SaSTL formulas, 
we define a series of templates using structured language learning from the existing city requirements. For example, one template is written as, ``{The {<aggregation operator>} <entity> within {<d> km} of {<spatial operator> <PoIs>} should {<temporal operator>} be {<compare> <parameter>} {within the next <t> hours} ({from <m>th hour to <n>th hour})}''. Using this template, a city
administrator can easily specify an environmental requirement (and encourage quantitative details) as 
``{The <average> <air quality> within <1> mile of all <parks> should <always> be <above> <good> in the <next 3 hours>.}'' Further details on the templates are out of scope for this paper. 


In addition, we develop a prototype tool for the SaSTL monitor, the interface of which is shown in \figref{fig:tool}. 
To start with, users select the areas (such as a city, or a particular area of the city) to monitor, then choose the important labels that a requirement is involved with, such as schools, parks, theaters, etc. 
Once selected, the important points of interest (PoIs) are shown on the map. This helps users define and verify the monitoring locations. If a location or label is not included, users are also able to add them with their GPS coordinates.  
The data of the city states collected from sensors across temporal and spatial domains are introduced to the monitor in the Data section. 
As the next important step, users specify all requirements in the requirement section. Users first select the template and then choose/fill in the essential part using the structured template language. To be noted, the entities and spatial ranges correspond to the available data variables and PoIs inputs from the areas and data sections, respectively.
Moreover, users are also able to use the advanced features to input the city requirements in the format of the SaSTL formal formulas directly.  
The map displays the locations of the specified labels and sensors. Users can enlarge the map to check the distribution of sensors and PoIs and revise the requirements accordingly. 
With all the data and requirements well defined, users can start the monitor in order to check if the incoming data from the smart city satisfies the requirements. The results are displayed for each requirement with a Boolean value. 





\begin{algorithm}
\tablefontsize
  \SetKwFunction{Monitor}{Monitor}
  \SetKwProg{Fn}{Function}{:}{}
  \Fn{\Monitor{$\varphi,\omega, t, l, G$}}{
      \SetKwInOut{Input}{Input}
      \SetKwInOut{Output}{Output}
      \SetKwFor{Case}{Case}{}{}
      \Input{SaSTL Requirement $\varphi$, Signal $\omega$, Time $t$, Location $l$, weighted undirected graph $G$}
      
      \Output{Satisfaction Value (Boolean value)}
      
      \Begin{
            \Switch{$\varphi$} {
                   \Case{$p$}{
                        \Return $\pi_{p}[t,l]$;
                   }

                   \Case{$x\sim c$}{
                        \Return $\pi_x(\omega)[t, l] \sim c$;
                   }

                   \Case{$\neg \varphi$}{
                        \Return $\neg$ Monitor($\varphi,\omega, t, l, G$);
                   }
 
                   \Case{$\varphi_1 \land \varphi_2$  \Comment*[r]{See \algref{alg:and} for an improved algorithm.} }{
                        \Return Monitor($\varphi_1,\omega, t, l, G$) 
                        $\land$ Monitor($\varphi_2,\omega, t, l, G$) 
                        % \If{$\mathsf{cost}(\varphi_1, l, G) \leq \mathsf{cost}(\varphi_2, l, G)$}{      
                        %     \If {$\neg$ Monitor($\varphi_1,\omega, t, l, G$)}{
                        %          \Return Monitor($\varphi_2,\omega, t, l, G$);
                        %     }
                        %     \Return True;
                        % }
                        % \If {$\neg$ Monitor($\varphi_2,\omega, t, l, G$)}{
                        %     \Return Monitor($\varphi_1,\omega, t, l, G$);
                        % }
                        % \Return True;
                    }
                    
                    \Case{$ \varphi_1 U_I \varphi_2$ 
                    \Comment*[r]{See \algref{alg:Until}.}
                    }{ 
                         \Return SatisfyUntil($\varphi_1,\varphi_2, I, \omega, t, l, G$);
                    }
 
                    % \Case{$ \varphi_1 S_I \varphi_2$}{
                    %      \Return SatisfySince($\varphi_1,\varphi_2, I, \omega, t, l, G$);
                    % }

                    \Case{$\ag^{\op} x \sim c$   \Comment*[r]{See \algref{alg:Aggregation}}. }
                    {
                          \Return Aggregate$(x, c, op, d_1, d_2, t, l, G)$;
                    }
                    
                    \Case{$\ct^{\op} \varphi \sim c$   \Comment*[r]{See \algref{alg:Counting} for the standard version, and \algref{alg:CountingPara} for an improved parallel version.}}
                    { 
                          \Return CountingNeighbours$(\varphi, c, op, d_1, d_2, t, l, G) $; 
                    }
           }
       }
    }
\caption{SaSTL monitoring algorithm Monitor({$\varphi,\omega, t, l, G$})}
\label{alg:sastl}
\end{algorithm}


\section*{Appendix B: Specification Examples}
We give two more examples on how to use SaSTL to specify real city requirements, especially for the temporal elements. 

\begin{example} [Dynamic Deadlines]
The first requirement in \tabref{tab:reqexamples} is, ``Limits vehicle idling to one minute adjacent to any school, pre-K to 12th grade, public or private, in the City of New York.''
The requirement is specified using the SaSTL syntax as,


% formula to be added


% \begin{equation*}

$$(\mathsf{Idle_{taxi}} \rightarrow \eventually_{[0,1]} \neg \mathsf{Idle_{taxi}}) \land \mathsf{ school}
\vspace{-0.5cm}$$
% \end{equation*}
\label{ex:sytaxddl}

\end{example}

We use $\eventually_{[0,1]}$ to specify the deadline (i.e., within 1 minute) in this formula, so that if a vehicle idling is detected (i.e., $\mathsf{Idle_{taxi}}$ is $\mathsf{True}$), then, it must not be idling within 1 minute, i.e., $\neg \mathsf{Idle_{taxi}}$ has to be satisfied within 1 minute. To clarify, in SaSTL, the time range $[0,1]$ is a relative time interval, which means that 1 minute counts from when $\mathsf{Idle_{taxi}}$ is $\mathsf{True}$. 
In addition, we use the propositional variable $p$ (i.e.,  ``$\land~\mathsf{school}$'') to specify that the locations are tagged as school.  

% In SaSTL, we are able to specify the average and the worst case of the traffic, by 
% $(\agr_{[0,0.5]}^{\avg} x_\mathsf{traffic} < \mathsf{Moderate} \land \agr_{[0,0.5]}^{\max} x_\mathsf{traffic} < \mathsf{Safe})$. By this way, it not only covers the values from multiple locations and also defines the average and worst performance to check at the same time. A more reasonable number and meaningful violations are detected under such a SaSTL requirement.

\begin{example} [Time Intervals]
The third requirement in \tabref{tab:reqexamples} is, 
``Prohibit sightseeing buses from using all bus lanes between the hours of 7:00 a.m. and 10:00 a.m. on weekdays'', is specified using the SaSTL syntax as, 

% $\always_{[7,10]} \mathcal{C}_{[0, +\infty]} (\mathsf{BusLane(sightseeing bus)} < \mathsf{Num(BusLane)}) 
%  \land \mathsf{weekday}$.

% \begin{equation*}
% \begin{split}
$$ \always_{[7,10]} \everywhere_{[0,1]} (\neg \mathsf{ssbus})\land \mathsf{buslane} $$
%  \end{split}
%  \hspace{-0.5cm}
% \end{equation*}

\label{ex:sytaxsdl}
\end{example}

Assuming we monitor the bus lanes all day (from 12am), here we first use ``$\always_{[7,10]}$ to specify the time interval. $\mathsf{ssbus}$ (i.e. $\mathsf{ssbus==True}$) denotes that the bus lane is occupied by sightseeing buses. Therefore, $\neg \mathsf{ssbus}$ indicates there is no sightseeing buses on any bus lane. 


\section*{Appendix C: Monitoring Algorithms}

We present SaSTL the monitoring algorithm 
$\mathsf{Monitor}$ $(\varphi,\omega, t, l, G)$ and Satisfaction of Until in \algref{alg:sastl} and \algref{alg:Until}, respectively. The parallelization of counting operator is presented in \algref{alg:CountingPara}.



\begin{algorithm}
\tablefontsize
 \SetKwFunction{CS}{SatisfyUntil}
  \SetKwProg{Fn}{Function}{:}{}
  \Fn{\CS{$\varphi_1,\varphi_2, I, \omega, t, l, G$}}{
      \Begin{
  
             \textbf{Boolean} f := True;
             
             \For {$t'\in (t + I) \cap \mathbb{T}$}
             {
                  \If {Monitor$(\varphi_2, \omega, t',l,G)$}{
                       f := True;
                      
                       \For {$t'' \in [t,t']$}{
                            f := f $ \wedge $ Monitor$(\varphi_1, \omega, t'', l, G)$;
                            
                            \If{($\neg f$)}{\textbf{break;}}
                       }
                       \If{($f$)}{\Return True;}
                   }
             }
             \Return False;
        }
  }
\caption{Satisfaction of $(\varphi_1 U_I \varphi_2, \omega)$}
\label{alg:Until}
\end{algorithm}



\begin{algorithm}
\tablefontsize
 \SetKwFunction{CS}{CountingNeighbours}
 \SetKwFunction{worker}{worker}
  \SetKwProg{Fn}{Function}{:}{}
  \Fn{\CS{$\varphi,op, d_1, d_2, \omega, t, l, G$}}{
      \Begin{
 
              paratasks = Queue();
            %   \For {$l' \in L^l_{[d_1,d_2]}$}{
              
              
            \For{$l' \in L^l_{[d_1,d_2]}$}{paratasks.add($l$)\;}
                
                results = Queue()\;
                
                \For{i in $1..\text{NumThreads}$}{
                Thread$_i$ $\leftarrow$ worker($\varphi,\omega, t, G$)\;
                }
                Wait()\;
                \Return op(results)\;
      }
}
  \Fn{\worker($\varphi,\omega, t, G$)}{
  \Begin{
               \textbf{Real} $v := 0$;
              
              \lIf{$op$ == "min"}
              {
                    $v := \infty $;
              }
              
              \lIf{$op$ == "max"}
              {
                  $v := - \infty $;
              }
\While{Num(tasks)>0}{
$l$ = paratasks.pop()\;
moni = Monitor($\varphi, \omega, t, l, G$)\;
v = op(v, moni)\;
}
%\If{$op$ == "avg"}{
 %                \Return $v\backslash |L^{l}_{[d_1,d_2]}|$;
  %           }
  results.add(v)
  }
}
            
\caption{Parallelization of Counting of $(x, op, d_1, d_2, \omega, t, l, G)$}
\label{alg:CountingPara}
% \vspace{-1em}
\end{algorithm}




\section*{Appendix D: Discussion}
\input{8_discussion.tex}
